# Supplementary material for: Fewer measurements from shadow tomography with $N$-representability conditions
Source: arXiv:2312.11715 source file (2023-12-18)
Supplement: Supplementary file 1 [file SI-2-RDM-Shadow-Tomography.pdf]

# Supplemental Material:
# Fewer measurements from shadow tomography with $N$-representability conditions

Irma Avdic and David A. Mazziotti*
*Department of Chemistry and The James Franck Institute,*
*The University of Chicago, Chicago, IL 60637 USA*
(Dated: Submitted December 18, 2023)

## ADDITIONAL DATA

TABLE S1: The Euclidean norm of the absolute error of the 2-RDM computed via sv2RDM and FCI with DQG conditions and the total energy (Hartree) for $H_5$ at 1.00 Å separation of H atoms, as a function of the number of shadows. The FCI energy is -2.65451697 Hartree and the v2RDM energy is -2.66447993 Hartree. The trace of the 2-RDM is set to one.

| Shadow number | sv2RDM energy (Hartree) | Euclidean norm |
|---|---|---|
| 1 | -2.66290104 | 0.04112581 |
| 3 | -2.66041116 | 0.02141652 |
| 5 | -2.65724632 | 0.00748939 |
| 7 | -2.65599787 | 0.00487635 |
| 9 | -2.65570427 | 0.00295221 |
| 11 | -2.65535044 | 0.00148801 |
| 13 | -2.65486205 | 0.00136300 |
| 15 | -2.65466665 | 0.00065789 |
| 17 | -2.65451697 | 0.00019911 |

TABLE S2: The Euclidean norm of the absolute error of the 2-RDM computed via sv2RDM and FCI with DQG conditions and the total energy (Hartree) for $H_6$ at 1.00 Å separation of H atoms, as a function of the number of shadows. The FCI energy is -3.23606628 Hartree and the v2RDM energy is -3.24407931 Hartree. The trace of the 2-RDM is set to one.

| Shadow number | sv2RDM energy (Hartree) | Euclidean norm |
|---|---|---|
| 1 | -3.24311939 | 0.03707779 |
| 3 | -3.24209910 | 0.02764575 |
| 5 | -3.2410106 | 0.02265639 |
| 7 | -3.23959706 | 0.00588822 |
| 9 | -3.23853874 | 0.00342319 |
| 11 | -3.23801925 | 0.00220432 |
| 13 | -3.23711953 | 0.00197898 |
| 15 | -3.23695956 | 0.00155529 |
| 17 | -3.23698907 | 0.00142037 |
| 19 | -3.23654421 | 0.00108701 |
| 21 | -3.23657486 | 0.00103899 |
| 23 | -3.23621790 | 0.00098648 |
| 25 | -3.23608306 | 0.00102677 |
| 27 | -3.23606628 | 0.00053637 |

TABLE S3: The Euclidean norm of the absolute error of the 2-RDM computed via sv2RDM and FCI with DQG conditions and the total energy (Hartree) for $H_7$ at 1.00 Å separation of H atoms, as a function of the number of shadows. The FCI energy is -3.73548753 Hartree and the v2RDM energy is -3.75371421 Hartree. The trace of the 2-RDM is set to one.

| Shadow number | sv2RDM energy (Hartree) | Euclidean norm |
|---|---|---|
| 1 | -3.75281205 | 0.05182792 |
| 3 | -3.75091323 | 0.03994524 |
| 5 | -3.74936700 | 0.03327169 |
| 7 | -3.74692069 | 0.03388806 |
| 9 | -3.74567433 | 0.03626628 |
| 11 | -3.74287558 | 0.01733036 |
| 13 | -3.74238856 | 0.01180265 |
| 15 | -3.74049734 | 0.00635232 |
| 17 | -3.73878198 | 0.00321046 |
| 19 | -3.73833913 | 0.00390605 |
| 21 | -3.73805165 | 0.00377233 |
| 23 | -3.73763877 | 0.00242160 |
| 25 | -3.73758537 | 0.00169237 |
| 27 | -3.73696228 | 0.00179318 |
| 29 | -3.73657142 | 0.00229616 |
| 31 | -3.73651338 | 0.00215099 |
| 33 | -3.73608461 | 0.00194354 |
| 35 | -3.73589811 | 0.00278908 |
| 37 | -3.73552761 | 0.00094593 |
| 39 | -3.73548753 | 0.00087722 |

* Electronic address: damazz@uchicago.edu

TABLE S4: The Euclidean norm of the absolute error of the 2-RDM computed via sv2RDM and FCI with DQG conditions and the total energy (Hartree) for $H_8$ at 1.00 Å separation of H atoms, as a function of the number of shadows. The FCI energy is -4.30757160 Hartree and the v2RDM energy is -4.32291185 Hartree. The trace of the 2-RDM is set to one.

| Shadow number | sv2RDM energy (Hartree) | Euclidean norm |
|---|---|---|
| 1 | -4.32215060 | 0.04800580 |
| 3 | -4.32091467 | 0.03894779 |
| 5 | -4.32005110 | 0.03874101 |
| 7 | -4.31909665 | 0.03042557 |
| 9 | -4.31794120 | 0.02706046 |
| 11 | -4.31727535 | 0.01668232 |
| 13 | -4.31613371 | 0.01631687 |
| 15 | -4.31452050 | 0.01425402 |
| 17 | -4.31392850 | 0.00914502 |
| 19 | -4.31370491 | 0.00545305 |
| 21 | -4.31201186 | 0.00558218 |
| 23 | -4.31194606 | 0.00820932 |
| 25 | -4.31079046 | 0.00416006 |
| 27 | -4.30974452 | 0.00243050 |
| 29 | -4.30956950 | 0.00275149 |
| 31 | -4.30946945 | 0.00181368 |
| 33 | -4.30945765 | 0.00233200 |
| 35 | -4.30934339 | 0.00164151 |
| 37 | -4.30913381 | 0.07192697 |
| 39 | -4.30892749 | 0.00140248 |
| 41 | -4.30869830 | 0.00134430 |
| 43 | -4.30842589 | 0.00129142 |
| 45 | -4.30820226 | 0.00156066 |
| 47 | -4.30794389 | 0.00117327 |
| 49 | -4.30758121 | 0.00088410 |
| 51 | -4.30757166 | 0.00063863 |
| 53 | -4.30757159 | 0.00064255 |

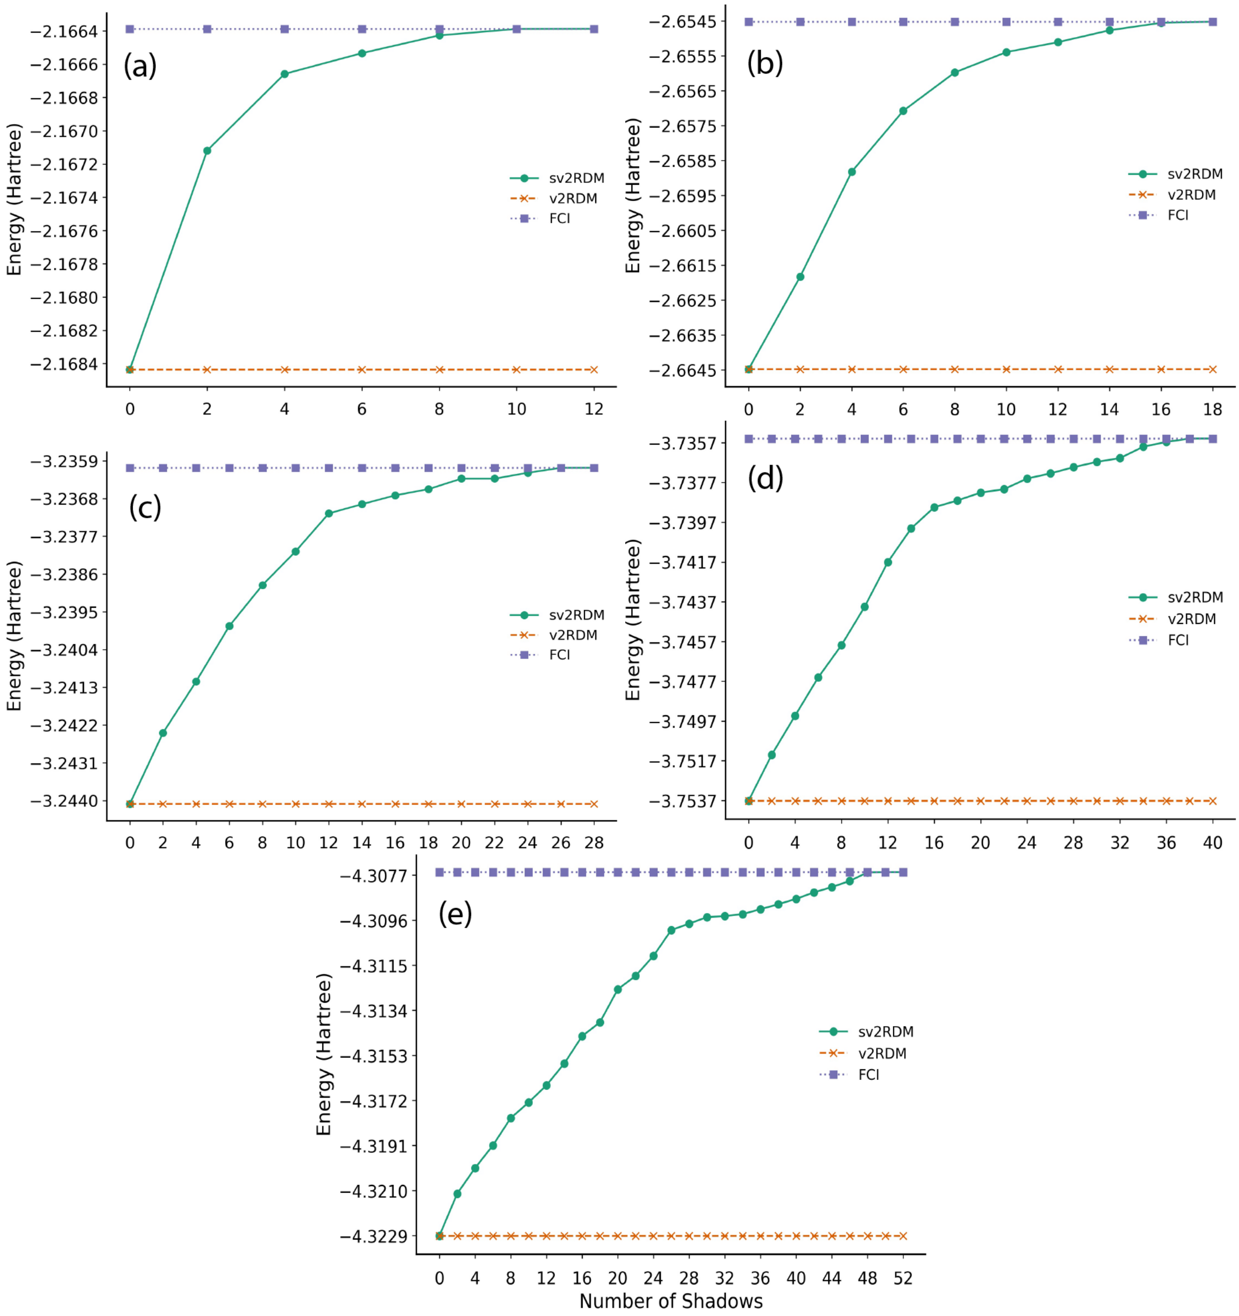


FIG. S1: Total ground state energy (Hartree) of (a) $H_4$, (b) $H_5$, (c) $H_6$, (d) $H_7$, and (e) $H_8$ with equally spaced H atoms, as a function of the number of shadows. By default, v2RDM and sv2RDM include D, Q, and G conditions. The sv2RDM energy converges *exactly* to the FCI energy in the noiseless environment.
